# Supplementary material for: Speech-to-Speech Translation For A Real-world Unwritten Language
Source: arXiv:2211.06474 source file (2022-11-11)
Supplement: Supplementary file 1 [file appendix.tex]

\section{Mined data quality}
\label{sec:appendix}
\al{tentative}

We evaluated our speech student encoders for Hokkien with similarity search on TAT devh1 set. Hokkien speech utterances are encoded with the speech encoder, English text transcripts are encoded with the text encoder. For each audio utterance,  we search for the closest transcript with respect to our margin-based similarity score. An error is counted when an audio is wrongly matched with some text. We provide the error rate in \% in Table \ref{tab:simsearch}. We notice that using our newly trained text encoder as teacher boosts the performance of the speech encoder.

\begin{table}
\centering
\begin{tabular}{ll}
\hline
Teacher & Error rate\\
\hline
Laser Original & 5.61 \\
XML-R Text Student   & 2.04 \\    
\hline
\end{tabular}
\caption{Similarity search error rates (in \%) of Hokkien speech against English text on 196 deduplicated instances of TAT-devh1 set.}
\label{tab:simsearch}
\end{table}
